# Supplementary material for: Substrate effects on charged defects in two-dimensional materials
Source: arXiv:1908.05208 source file (2019-08-14)
Supplement: Supplementary file 1 [file SI.pdf]

# Supplemental Material for "Substrate effects on charged defects in two-dimensional materials"

Dan Wang and Ravishankar Sundararaman*
*Department of Materials Science and Engineering, Rensselaer Polytechnic Institute, 110 8th Street, Troy, NY*
(Dated: August 8, 2019)

## ANISOTROPIC DIELECTRIC FUNCTION FOR CHARGE CORRECTION

Energy correction for charged defects in 2D materials requires the anisotropic dielectric tensor, $\bar{\epsilon}^{2D}(z)$, which has two independent components for materials like hBN and $MoS_2$ which are in-plane isotropic. Specifically, we need to determine $\epsilon_{zz}^{2D}(z) = \epsilon_{\perp}^{2D}(z)$ and $\epsilon_{xx}^{2D}(z) = \epsilon_{yy}^{2D}(z) = \epsilon_{\parallel}^{2D}(z)$. Following Ref. 1, we calculate $\epsilon_{\perp}^{2D}(z)$ from the difference in net electrostatic potential profiles between two calculations with different electric fields applied along the $z$-direction, as described in detail in Ref. 2. This yields the spatial distribution of the out-of-plane dielectric response fully from first principles.

We assume that the in-plane dielectric response has the same spatial profile as $\epsilon_{\perp}^{2D}(z)$, and determine it based on the sum rule constraint[3]

$$\int dz \epsilon_{\parallel}^{2D}(z) = L_z \epsilon_{\parallel}^{2D} \tag{1}$$

where $\epsilon_{\parallel}^{2D}$ is the total in-plane dielectric function for the unit cell calculated by density functional perturbation theory. This construction ensures a physical extent of the in-plane polarization without introducing additional spatial parameters as in Ref. 3, and the constraint ensures a correct overall magnitude of in-plane polarization. See Refs. 1 and 2 for additional details. For each calculation involved in determining $\epsilon^{2D}(z)$, we use the same cell lengths $L_z$ normal to the 2D material i.e., 30 Å for $MoS_2$ and 16 Å for hBN.

## CONTINUUM MODEL DETAILS

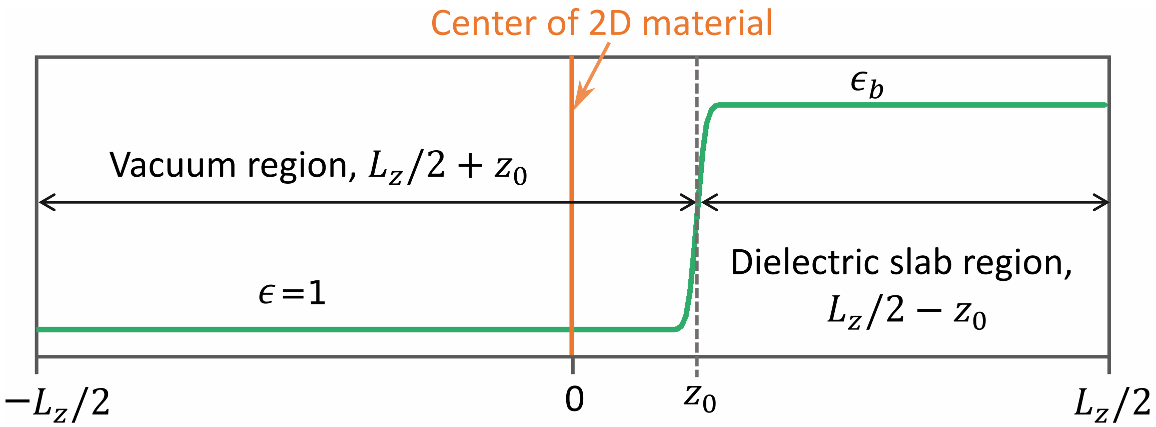


FIG. S1. Schematic illustration of the continuum-model dielectric function (green line) separating the substrate dielectric slab and vacuum regions, relative to the 2D material centered at $z = 0$ (orange line).

TABLE S1. Thickness of vacuum region and dielectric slab for $MoS_2/SiO_2$, $hBN/SiO_2$, and hBN/Diamond. Here, $\sigma$ controls the transition width of the shape function as discussed in the main text. The ionization energies (IE) of substitution defects in $MoS_2$ converge fully for $\sigma \leq 0.3$ Å.

| System | $\sigma$ (Å) | $z_0$ (Å) | $L_z$ (Å) | Vacuum region $L_z/2 + z_0$ (Å) | Slab region $L_z/2 - z_0$ (Å) | IE (eV) $Re_{Mo}$ | IE (eV) $Nb_{Mo}$ |
|---|---|---|---|---|---|---|---|
| $MoS_2/SiO_2$ | 0.125 | 3.44 | 30 | 18.44 | 11.56 | 0.296 | 0.365 |
| | 0.15 | 3.45 | | 18.45 | 11.55 | 0.296 | 0.365 |
| | 0.20 | 3.47 | | 18.47 | 11.53 | 0.296 | 0.364 |
| | 0.25 | 3.50 | | 18.50 | 11.50 | 0.295 | 0.364 |
| | 0.30 | 3.53 | | 18.53 | 11.47 | 0.294 | 0.364 |
| | 0.35 | 3.56 | | 18.56 | 11.44 | 0.286 | 0.367 |
| | 0.42 | 3.60 | | 18.60 | 11.40 | 0.284 | 0.355 |
| $MoS_2/SiO_2$ | 0.2 | 3.47 | 30 | 18.47 | 11.53 | | |
| $hBN/SiO_2$ | | 2.11 | 16 | 10.11 | 5.89 | | |
| hBN/Diamond | | 1.96 | 16 | 9.96 | 6.04 | | |

## IONIZATION ENERGY COMPARISONS AND NEUTRAL FORMATION ENERGY

TABLE S2. Ionization energies of $Re_{Mo}$ and $Nb_{Mo}$ in $MoS_2$ and $MoS_2/SiO_2$. Values from previous studies with explicit substrate are shown for comparison. Bold numbers denote the reduction in ionization energy.

| Ionization energy (eV) | $Nb_{Mo}$ | | | $Re_{Mo}$ | | |
|---|---|---|---|---|---|---|
| | $MoS_2$ | $MoS_2/SiO_2$ | *difference* | $MoS_2$ | $MoS_2/SiO_2$ | *difference* |
| Ref. 40[4] | 0.52 | 0.39 | **0.13** | 0.53 | 0.38 | **0.15** |
| Ref. 24[5] | 0.55 | - | - | 0.45 | - | - |
| Present work | 0.51 | 0.36 | **0.15** | 0.40 | 0.30 | **0.10** |

TABLE S3. Ionization energies of $C_B$, $V_N$ and $N_BV_N$ in $hBN/SiO_2$ and hBN/Diamond, obtained by explicit-substrate and continuum model calculations.

| Ionization energies (eV) | $C_B$ (donor) | | $V_N$ (donor) | | $N_BV_N$ (donor) | | $V_N$ (acceptor) | |
|---|---|---|---|---|---|---|---|---|
| | Explicit | Model | Explicit | Model | Explicit | Model | Explicit | Model |
| $hBN/SiO_2$ | 2.30 | 2.20 | 2.65 | 2.55 | 3.75 | 3.63 | - | - |
| hBN/Diamond | 2.08 | 1.92 | 2.38 | 2.28 | - | - | 3.66 | 3.50 |

TABLE S4. Neutral formation energies of $C_B$, $V_N$ and $N_BV_N$ in free-standing hBN, hBN/$SiO_2$ and hBN/Diamond under B-rich and N-rich conditions, obtained with explicit-substrate and continuum model calculations.

| B-rich condition (eV) | $C_B$ | | $V_N$ | | $N_BV_N$ | |
|---|---|---|---|---|---|---|
| | Explicit | Model | Explicit | Model | Explicit | Model |
| Free-standing hBN | 4.25 | - | 5.10 | - | 10.28 | - |
| hBN/$SiO_2$ | 4.28 | 4.25 | 5.15 | 5.10 | 10.35 | 10.28 |
| hBN/Diamond | 4.27 | 4.23 | 5.26 | 5.10 | - | - |
| N-rich condition (eV) | $C_B$ | | $V_N$ | | $N_BV_N$ | |
| | Explicit | Model | Explicit | Model | Explicit | Model |
| Free-standing hBN | 1.68 | - | 7.67 | - | 7.71 | - |
| hBN/$SiO_2$ | 1.71 | 1.68 | 7.72 | 7.67 | 7.78 | 7.71 |
| hBN/Diamond | 1.70 | 1.66 | 7.83 | 7.67 | - | - |

TABLE S5. Comparison of ionization energy reduction due to substrate predicted by self-consistent continuum model calculations for each defect, with single non-self-consistent estimates for each 2D material - substrate combination using the same continuum model based on Eq. 7 in the main text (shown in the final column in **bold** text).

| Donors | $Re_{Mo}$ | $C_B$ | $V_N$ | $N_BV_N$ | $Si_BV_N$ | $C_BV_N$ | $Si_NC_NV_B$ | $Si_BC_BV_N$ | $(O_B)_2V_N$ | Eq. 7 |
|---|---|---|---|---|---|---|---|---|---|---|
| $\Delta IE_{MoS_2/SiO_2}$ (eV) | 0.10 | - | - | - | - | - | - | - | - | **0.10** |
| $\Delta IE_{hBN/SiO_2}$ (eV) | - | 0.32 | 0.31 | 0.31 | 0.33 | 0.31 | 0.32 | 0.33 | 0.31 | **0.32** |
| $\Delta IE_{hBN/Diamond}$ (eV) | - | 0.60 | 0.59 | 0.59 | 0.64 | 0.58 | 0.60 | 0.62 | 0.58 | **0.60** |
| Acceptors | $Nb_{Mo}$ | $C_N$ | $V_N$ | $N_BV_N$ | $Si_BV_N$ | $C_NV_B$ | $Si_NC_NV_B$ | $Si_BC_BV_N$ | $(O_B)_2V_N$ | Eq. 7 |
| $\Delta IE_{MoS_2/SiO_2}$ (eV) | 0.15 | - | - | - | - | - | - | - | - | **0.14** |
| $\Delta IE_{hBN/SiO_2}$ (eV) | - | 0.28 | 0.29 | 0.28 | 0.27 | 0.29 | 0.27 | 0.28 | 0.29 | **0.27** |
| $\Delta IE_{hBN/Diamond}$ (eV) | - | 0.51 | 0.51 | 0.50 | 0.47 | 0.51 | 0.47 | 0.49 | 0.52 | **0.48** |

* sundar@rpi.edu


[1] F. Wu, A. Galatas, R. Sundararaman, D. Rocca, and Y. Ping, Phys. Rev. Mater. **1**, 071001 (2017).

[2] R. Sundararaman and Y. Ping, J. Chem. Phys. **146**, 104109 (2017).

[3] H.-P. Komsa and A. Pasquarello, Phys. Rev. Lett. **110**, 095505 (2013).

[4] J.-Y. Noh, H. Kim, M. Park, and Y.-S. Kim, Phys. Rev. B **92**, 115431 (2015).

[5] D. Wang, D. Han, D. West, N.-K. Chen, S.-Y. Xie, W. Q. Tian, V. Meunier, S. Zhang, and X.-B. Li, npj Comput. Mater. **5**, 8 (2019).
